# Supplementary material for: Stabilized isogeometric formulation of the Stokes problem on overlapping patches
Source: arXiv:2305.20021 source file (2023-09-21)
Supplement: Supplementary file 1 [file appendix.tex]

\documentclass[class=elsarticle, crop=false]{standalone}

\begin{document}
%------------------------------------------------------------------------------------------------------------------------------
%------------------------------------------------------------------------------------------------------------------------------	
\section{Technical proofs}\label{appendix:A1}
\begin{proof}[Proof of Theorem~\ref{thm:wellposedness}]
In order to prove~\eqref{wellposed:eq1}, let us show that there exist $c_1,c_2>0$ such that, for every $\left(\vv_h, q_h,\bmu_h \right)\in V_h\times\overline Q_h\times\Lambda_h$, there exists $\left(\w_h,r_h,\bm\eta_h \right)\in V_h\times\overline Q_h\times\Lambda_h$ such that $\overline{\mathcal A}_h\left( \left( \w_h,r_h,\bm\eta_h\right) ;\left(\vv_h,q_h,\bm\eta_h\right)\right) \ge c_1 \vertiii{\left(\vv_h,q_h,\bmu_h\right)}^2$ and $\vertiii{\left(\w_h,r_h,\bm\eta_h\right)}\le c_2 \vertiii{\left(\vv_h,q_h,\bmu_h\right)}$. Let us take $\left(\vv_h,q_h,\bmu_h\right)\in V_h\times\overline Q_h\times\Lambda_h$. It holds
\begin{align*}
&\overline{\mathcal A}_h \left( \left( \vv_h,-q_h,-\bmu_h \right) ;\left( \vv_h,q_h,\bmu_h\right) \right) = \sum_{i=0}^N\norm{D\vv_i}^2_{L^2(\Omega_i)}\\
&+\sum_{i=1}^N\sum_{j=0}^{i-1} \gamma^{-1} \left[ \norm{\h^{\frac{1}{2}}\left(-\bmu_h +\langle q_h\n \rangle_t\right)}^2_{L^2(\Gamma_{ij})} - \norm{\h^{\frac{1}{2}}\langle DR_{ij}^v(\vv_h)\n\rangle_t}^2_{L^2(\Gamma_{ij})}  \right] .
\end{align*}
%Notice that
%\begin{align*}
%\gamma^{-1}\norm{\h^{\frac{1}{2}}\left(-\bmu_h +\langle q_h\n \rangle_t\right)}^2_{L^2(\Gamma_{ij})} = & \gamma^{-1} \left(\norm{\h^{\frac{1}{2}}\bmu_h}^2_{L^2(\Gamma_{ij})} -2\int_{\Gamma_{ij}}\h \bmu_h \langle q_h\n\rangle_{t}+\norm{\h^{\frac{1}{2}}\langle q_h\n \rangle_t}^2_{L^2(\Gamma_{ij})}\right). 
%\end{align*}
Hence, by using Proposition~\ref{proposition_stability_velocity} and choosing $\gamma>0$ large enough,
\begin{equation}\label{appendix:eq:runliang1}
\begin{aligned}
\overline{\mathcal A}_h \left(\left( \vv_h,-q_h,-\bmu_h\right);\left(\vv_h,q_h,\bmu_h\right)\right)	
\ge&  \left(1-C\gamma^{-1}\right)\sum_{i=0}^N \norm{D\vv_i}^2_{L^2(\Omega_i)}
+ \gamma^{-1}\sum_{i=1}^N\sum_{j=0}^{i-1}\norm{\h^{\frac{1}{2}}\left(-\bmu_h+ \langle q_h\n\rangle_t\right)}^2_{L^2(\Gamma_{ij})} \\
\ge & \frac{1}{2}  \sum_{i=0}^N\norm{D\vv_i}^2_{L^2(\Omega_i)} +\gamma^{-1}\sum_{i=1}^N\sum_{j=0}^{i-1}\norm{\h^{\frac{1}{2}}\left(-\bmu_h+ \langle q_h\n\rangle_t\right)}^2_{L^2(\Gamma_{ij})}.
\end{aligned}	
\end{equation}
Now, let $\w_h^q\in V_h$ be the supremizer of Lemma~\ref{lemma:is}. Since $b_0(\w_h^q,q_h)\ge C\norm{q_h}^2_{0,h}$, we have
\begin{equation}\label{wellposed:eq3}
\begin{aligned}
\overline{\mathcal A}_h\left(\left(\w_h^q,0,\bm 0\right);\left(\vv_h,q_h,\bmu_h\right)\right)
\ge & \sum_{i=0}^N\int_{\Omega_i} D\vv_i:D\w_i^p  +C  \norm{q_h}^2_{0,h} + \sum_{i=1}^N \sum_{j=0}^{i-1}\int_{\Gamma_{ij}} \bmu_h [\w_h^q]\\
& - \sum_{i=1}^N \sum_{j=0}^{i-1}\gamma^{-1} \int_{\Gamma_{ij}}\h \langle DR_{ij}^v(\vv_h)\n\rangle_t \langle DR_{ij}^v(\w_h^q)\n\rangle_t\\
&+  \sum_{i=1}^N \sum_{j=0}^{i-1} \gamma^{-1} \int_{\Gamma_{ij}}\h \left( -\bmu_h + \langle q_h\n\rangle_t\right) \langle DR_{ij}^v(\w_h^q)\n\rangle_{t}.
\end{aligned}	
\end{equation}
By the Cauchy-Schwarz inequality
\begin{align*}
\sum_{i=1}^N \sum_{j=0}^{i-1} &	\int_{\Gamma_{ij}} \h \langle DR_{ij}^v(\vv_h)\n\rangle_t \langle DR^v_h(\w_h^q)\n\rangle_t\\
\le  & \sum_{i=1}^N \sum_{j=0}^{i-1} \norm{ \h^{\frac{1}{2}}\langle DR_{ij}^v(\vv_h)\n\rangle_t}_{L^2(\Gamma_{ij})}\norm{\h^{\frac{1}{2}}\langle DR_{ij}^v(\w_h^q)\n\rangle_t}_{L^2(\Gamma_{ij})},\\
\sum_{i=1}^N \sum_{j=0}^{i-1} &	\abs{ \int_{\Gamma_{ij}}\h \left(-\bmu_h+\langle q_h\n\rangle_t\right) \langle DR_{ij}^v(\w_h^q)\n  \rangle_{t}}\\
\le&\sum_{i=1}^N \sum_{j=0}^{i-1}  \norm{\h^{\frac{1}{2}} \left(-\bmu_h +\langle q_h\n\rangle_t \right)}_{L^2(\Gamma_{ij})}
\norm{\h^{\frac{1}{2}}\langle DR_{ij}^v(\w_h^q)\n\rangle_t}_{L^2(\Gamma_{ij})}.
\end{align*}	
By using Young's inequality, for $s,\delta>0$, Proposition~\ref{proposition_stability_velocity} and the construction of $\w_h^q$ in the proof of Lemma~\ref{lemma:is}, there exists $C_1>0$ such that
\begin{align*}
\sum_{i=1}^N \sum_{j=0}^{i-1}\gamma^{-1}\int_{\Gamma_{ij}} \h\langle DR_{ij}^v(\vv_h)\n\rangle_t \langle DR^v_{ij}(\w_h^q)\n\rangle_t  	\ge & -\frac{C_1}{2\gamma s} \sum_{i=0}^N\norm{D\vv_i}^2_{L^2(\Omega_i)} - \frac{sC_1}{2\gamma}\norm{q_h}^2_{0,h}, \\
\sum_{i=1}^N \sum_{j=0}^{i-1} \gamma^{-1}\int_{\Gamma_{ij}} \h \left(-\bmu_h+\langle q_h\n\rangle_t\right) \langle DR_{ij}^v(\w_h^q)\n  \rangle_{t} \ge & -\frac{C_1}{2\gamma\delta}\sum_{i=1}^N \sum_{j=0}^{i-1} \norm{\h^{\frac{1}{2}}\left(-\bmu_h+\langle q_h\n\rangle_t\right))}_{L^2(\Gamma_{ij})}^2\\
& -\frac{\delta C_1}{2\gamma} \norm{q_h}^2_{0,h}.
\end{align*}	
From the Cauchy-Schwarz inequality, the construction of $\w_h^q$, and Young's inequality, there exists $C_2>0$ such that, for $\eps>0$,
\begin{align*}
\sum_{i=0}^N \int_{\Omega_i}D\vv_i:D\w_i^p \ge -\frac{C_2}{2\eps} \sum_{i=0}^N \norm{D\vv_i}^2_{L^2(\Omega_i)} - \frac{\eps C_2}{2} \norm{q_h}^2_{0,h}.
\end{align*}	
In an analogous fashion, there exists $C_3>0$ such that, for $r>0$,
\begin{align*}
\sum_{i=1}^N \sum_{j=0}^{i-1}	\int_{\Gamma_{ij}} \bmu_h [\w_h^q] \ge -\frac{C_3}{2r} \sum_{i=1}^N \sum_{j=0}^{i-1} \norm{\mathsf h^{\frac{1}{2}}\bmu_h}^2_{L^2(\Gamma_{ij})} - \frac{rC_3 }{2} \norm{q_h}^2_{0,h}.
\end{align*}
Let us go back to~\eqref{wellposed:eq3}. We have
\begin{align*}
\overline{\mathcal A}_h& \left( \left(\w_h^q,0,\bm 0 \right)  ; \left(\vv_h,q_h,\bmu_h\right)\right)\ge -\frac{C_2}{2\eps} \sum_{i=0}^N\norm{D\vv_i}^2_{L^2(\Omega_i)}-\frac{\eps C_2}{2}\norm{q_h}^2_{0,h} +C\norm{q_h}^2_{0,h}\\
&-\frac{C_3}{2r}\sum_{i=1}^N \sum_{j=0}^{i-1}\norm{\h^{\frac{1}{2}}\bmu_h}^2_{L^2(\Gamma_{ij})}
- \frac{r C_3}{2}\norm{q_h}^2_{0,h}
-\frac{C_1 }{2\gamma s}\sum_{i=0}^N\norm{D\vv_i}^2_{L^2(\Omega_i)}\\
& - \frac{s C_1}{2\gamma}\norm{q_h}^2_{0,h}
- \frac{C_1}{2\gamma\delta}\sum_{i=1}^N\sum_{j=0}^{i-1} \norm{\h^{\frac{1}{2}} \left(-\bmu_h+\langle q_h\n\rangle_t \right)}_{L^2(\Gamma_{ij})} - \frac{\delta C_1 }{2\gamma}\norm{q_h}^2_{0,h}\\
= &\left( C-\frac{\eps C_2}{2}-\frac{r C_3}{2}-\frac{s C_1}{2\gamma} - \frac{\delta C_1 }{2\gamma}\right)\norm{q_h}^2_{0,h} + \left( -\frac{C_2}{2\eps}-\frac{C_1 }{2\gamma s}\right)\sum_{i=0}^N \norm{D\vv_i}^2_{L^2(\Omega_i)}\\
& - \frac{C_1}{2\gamma\delta} \sum_{i=1}^N\sum_{j=0}^{i-1}\norm{\h^{\frac{1}{2}}\left(-\bmu_h+\langle q_h\n\rangle \right)}^2_{L^2(\Gamma_{ij})} - \frac{C_3}{2r} \sum_{i=1}^N\sum_{j=0}^{i-1}\norm{\h^{\frac{1}{2}} \bmu_h}^2_{L^2(\Gamma_{ij})}.
\end{align*}
Let $\eps,r,s,\delta>0$ be small enough such that $\displaystyle C-\frac{\eps C_2}{2}-\frac{r C_3}{2}-\frac{s C_1}{2\gamma} - \frac{\delta C_1 }{2\gamma}\ge \frac{C}{2}$. Hence, there exist $C_4, C_5, C_6 >0$ such that
\begin{equation}\label{appendix:eq:runliang2}
\begin{aligned}
\overline{\mathcal A}_h&\left(\left(\w_h^q,0,\bm 0\right);\left(\vv_h,q_h,\bmu_h \right)\right)\ge \frac{C}{2} \norm{q_h}^2_{0,h}- C_4 \sum_{i=0}^N \norm{D\vv_i}^2_{L^2(\Omega_i)}\\
& -  C_5 \sum_{i=1}^N \sum_{j=0}^{i-1} \norm{\h^{\frac{1}{2}}\left( -\bmu_h+\langle q_h\n\rangle_t\right)}^2_{L^2(\Gamma_{ij})}
-C_6\sum_{i=1}^N \sum_{j=0}^{i-1}\norm{\h^{\frac{1}{2}}\bmu_h}^2_{L^2(\Gamma_{ij})}.
\end{aligned}
\end{equation}
Let $P_h:\bigoplus_{0\le j<i\le N} L^2(\Gamma_{ij})\to \Lambda_h$ be the $L^2$-orthogonal projection. From condition~\eqref{condition:multiplier_space}, we have $\h^{-1}\restr{[\vv_h]}{\Gamma_{ij}}=\restr{P_h \h^{-1}[\vv_h]}{\Gamma_{ij}}$, for every $0\le j<i\le N$. Therefore, from the Cauchy-Schwartz inequality, we have
\begin{align*}
\overline{\mathcal A}_h  \left( \left( \bm 0,0, P_h\h^{-1}[\vv_h] \right) ;\left(\vv_h,q_h,\bmu_h\right)\right)
\ge & \sum_{i=1}^N\sum_{j=0}^{i-1}  \norm{\h^{-\frac{1}{2}}[\vv_h]}^2_{L^2(\Gamma_{ij})}\\
&-\gamma^{-1}\bigg( \sum_{i=1}^N\sum_{j=0}^{i-1} \norm{\h^{\frac{1}{2}}\langle DR_{ij}^v(\vv_h)\n\rangle_t}_{L^2(\Gamma_{ij})} \norm{\h^{-\frac{1}{2}}[\vv_h]}_{L^2(\Gamma_{ij})}\\
& + \sum_{i=1}^N\sum_{j=0}^{i-1} \norm{\h^{\frac{1}{2}}\left( -\bmu_h+\langle q_h\n\rangle_t \right)}_{L^2(\Gamma_{ij})} \norm{\h^{-\frac{1}{2}}[\vv_h]}_{L^2(\Gamma_{ij})}\bigg).
\end{align*}
By Proposition~\ref{proposition_stability_velocity} and Young's inequality, there exists $C_7>0$ such that, for $a,b>0$,
\begin{align*}
- \sum_{i=1}^N\sum_{j=0}^{i-1} \norm{\h^{\frac{1}{2}}\langle  DR^v_h (\vv_h)\n\rangle_t}_{L^2(\Gamma_{ij})}\norm{\h^{-\frac{1}{2}}[\vv_h]}_{L^2(\Gamma_{ij})} \ge& -\frac{C_7 }{2a} \sum_{i=0}^N \norm{D \vv_i}^2_{L^2(\Omega_i)}\\
& - \frac{aC_7}{2} \sum_{i=1}^N\sum_{j=0}^{i-1} \norm{\h^{-\frac{1}{2}}[\vv_h]}^2_{L^2(\Gamma_{ij})},\\
- \sum_{i=1}^N\sum_{j=0}^{i-1} \norm{\h^{\frac{1}{2}}\left(-\bmu_h+\langle q_h \n \rangle_t\right)}_{L^2(\Gamma_{ij})}\norm{\h^{-\frac{1}{2}}[\vv_h]}_{L^2(\Gamma_{ij})}\ge& -\frac{1}{2b}  \sum_{i=1}^N\sum_{j=0}^{i-1} \norm{\h^{\frac{1}{2}}\left( -\bmu_h+\langle q_h\n\rangle_t\right)}^2_{L^2(\Gamma_{ij})}\\
&- \frac{b}{2}  \sum_{i=1}^N\sum_{j=0}^{i-1}\norm{\h^{-\frac{1}{2}}[\vv_h]}^2_{L^2(\Gamma_{ij})}.
\end{align*}
Thus,
\begin{equation*}
\begin{aligned}
\overline{\mathcal A}_h&\left( \left(\bm 0,0P_h\h^{-1}[\vv_h]\right);\left(\vv_h,q_h,\bmu_h\right)\right) \ge \left( 1-\frac{aC_7}{2\gamma}-\frac{b}{2\gamma}\right)  \sum_{i=1}^N\sum_{j=0}^{i-1} \norm{\h^{-\frac{1}{2}}[\vv_h]}^2_{L^2(\Gamma_{ij})}\\
& - \frac{C_7}{2a\gamma} \sum_{i=0}^N\norm{D\vv_i}^2_{L^2(\Omega_i)}-\frac{1}{2b\gamma}  \sum_{i=1}^N\sum_{j=0}^{i-1} \norm{\h^{\frac{1}{2}}\left(-\bmu_h+\langle q_h\n\rangle_t \right)}^2_{L^2(\Gamma_{ij})}.
\end{aligned}
\end{equation*}
Let us choose $a,b>0$ small enough such that $\displaystyle 1-\frac{aC_7}{2\gamma}-\frac{b}{2\gamma}\ge \frac{1}{2}$. Hence, there exist $C_8,C_9>0$ such that
\begin{equation}\label{appendix:eq:runliang3}
\begin{aligned}
\overline{\mathcal A}_h\left( \left(\bm 0,0,P_h\h^{-1}[\vv_h]\right);\left(\vv_h,q_h,\bmu_h\right)\right) \ge & \frac{1}{2}  \sum_{i=1}^N\sum_{j=0}^{i-1} \norm{\h^{-\frac{1}{2}}[\vv_h]}^2_{L^2(\Gamma_{ij})}
-C_8 \sum_{i=0}^N\norm{D\vv_i}^2_{L^2(\Omega_i)}\\
&-C_9  \sum_{i=1}^N\sum_{j=0}^{i-1} \norm{\h^{\frac{1}{2}}\left(-\bmu_h+\langle q_h\n\rangle_t \right)}^2_{L^2(\Gamma_{ij})}.
\end{aligned}
\end{equation}	
Let us put together~\eqref{appendix:eq:runliang1},~\eqref{appendix:eq:runliang2},~\eqref{appendix:eq:runliang3}. For $k,\eta>0$, we have
\begin{align*}
\overline{\mathcal A}_h&\left(\left( \vv_h + k \w^q_h,-q_h,-\bm\mu_h+\eta P_h \h^{-1} [\vv_h] \right) ;\left( \vv_h,q_h,\bmu_h\right)\right) 
\ge  \left( \frac{1}{2}-kC_4 -\eta C_8\right) \sum_{i=0}^N \norm{D\vv_i}^2_{L^2(\Omega_i)}\\
&+ \left(\frac{1}{\gamma}-kC_5-\eta C_9 \right) \sum_{i=1}^N \sum_{j=0}^{i-1} \norm{\h^{\frac{1}{2}}\left(-\bm\mu_h +\langle q_h\n\rangle_t\right)}^2_{L^2(\Gamma_{ij})} 
+ \frac{kC}{2} \norm{q_h}^2_{0,h}\\
& -kC_6 \sum_{i=1}^N \sum_{j=0}^{i-1}\norm{\h^{\frac{1}{2}}\bm\mu_h}^2_{L^2(\Gamma_{ij})} + \frac{\eta}{2} \sum_{i=1}^N \sum_{j=0}^{i-1} \norm{\h^{-\frac{1}{2}} [\vv_h]}^2_{L^2(\Gamma_{ij})} .
\end{align*}
From Proposition~\ref{prop_press_stability}, there exists $C_{10}>0$ such that
\begin{equation}\label{appendix:hongkong}
\begin{aligned}
\overline{\mathcal A}_h&\left(\left( \vv_h + k \w^q_h,-q_h,-\bm\mu_h+\eta P_h \h^{-1} [\vv_h] \right) ;\left( \vv_h,q_h,\bmu_h\right)\right) 
\ge  \left( \frac{1}{2}-kC_4 -\eta C_8\right) \sum_{i=0}^N \norm{D\vv_i}^2_{L^2(\Omega_i)}\\
&+ \left(\frac{1}{\gamma}-kC_5-\eta C_9 \right) \sum_{i=1}^N \sum_{j=0}^{i-1} \norm{\h^{\frac{1}{2}}\left(-\bm\mu_h +\langle q_h\n\rangle_t\right)}^2_{L^2(\Gamma_{ij})} 
+\frac{k}{4C_{10} }\sum_{i=1}^N\sum_{j=0}^{i-1} \norm{\h^{\frac{1}{2}}\langle q_h\rangle_t}^2_{L^2(\Gamma_{ij})}\\
&+ \frac{kC}{4} \norm{q_h}^2_{0,h} -kC_6 \sum_{i=1}^N \sum_{j=0}^{i-1}\norm{\h^{\frac{1}{2}}\bm\mu_h}^2_{L^2(\Gamma_{ij})} + \frac{\eta}{2} \sum_{i=1}^N \sum_{j=0}^{i-1} \norm{\h^{-\frac{1}{2}} [\vv_h]}^2_{L^2(\Gamma_{ij})} .
\end{aligned}
\end{equation}
Let $\displaystyle C_{11}:= \frac{4}{k C_{10}}$ and $\displaystyle C_{12}:=\frac{1}{\gamma}-kC_5-\eta C_9$, and observe that, by Young inequality, for any $\ell >0$,
\begin{equation*}
\norm{\h^{\frac{1}{2}}\left(-\bm\mu_h +\langle q_h\n\rangle_t\right)}^2_{L^2(\Gamma_{ij})} \ge 
(1-\ell) \norm{\h^{\frac{1}{2}}\langle q_h \n\rangle_t}^2_{L^2(\Gamma_{ij})} + (1-\frac{1}{\ell}) \norm{ \h^{\frac{1}{2}} \bmu_h}^2_{L^2(\Gamma_{ij})}.
\end{equation*}
%so that we can write
%\begin{align*}
%&C_{11}\sum_{i=1}^N\sum_{j=0}^{i-1} \norm{\h^{\frac{1}{2}}\langle q_h\rangle_t}^2_{L^2(\Gamma_{ij})} + C_{12} \sum_{i=1}^N \sum_{j=0}^{i-1} \norm{\h^{\frac{1}{2}}\left(-\bm\mu_h +\langle q_h\n\rangle_t\right)}^2_{L^2(\Gamma_{ij})}\\
%= &C_{12}  \sum_{i=1}^N \sum_{j=0}^{i-1} \left(  \left( \frac{C_{11}}{C_{12}} +1 \right) \norm{\h^{\frac{1}{2}} \langle q_h \n\rangle_t }^2_{L^2(\Gamma_{ij})}  + \norm{\h^{\frac{1}{2}}\bmu_h}^2_{L^2(\Gamma_{ij})} -2\int_{\Gamma_{ij}} \h^{\frac{1}{2}} \bmu_h \h^{\frac{1}{2}} \langle q_h \n\rangle_t \right).
%\end{align*}
%From the Cauchy-Schwartz and the Young inequalities, for $\ell >0$, it holds
%\begin{align*}
%-2 \int_{\Gamma_{ij}}\h^{\frac{1}{2}} \bmu_h \h^{\frac{1}{2}} \langle q_h \n\rangle_t \ge -\ell \norm{\h^{\frac{1}{2}}\langle q_h \n\rangle_t}^2_{L^2(\Gamma_{ij})} - \frac{1}{\ell} \norm{ \h^{\frac{1}{2}} \bmu_h}^2_{L^2(\Gamma_{ij})}.
%\end{align*}
By using $\norm{\h^{\frac{1}{2}}\langle q_h \n\rangle_t}^2_{L^2(\Gamma_{ij})} = \norm{\h^{\frac{1}{2}}\langle q_h \rangle_t}^2_{L^2(\Gamma_{ij})}$, we have
\begin{equation}\label{appendix:stress}
\begin{aligned}
&C_{11}\sum_{i=1}^N\sum_{j=0}^{i-1} \norm{\h^{\frac{1}{2}}\langle q_h\rangle_t}^2_{L^2(\Gamma_{ij})} + C_{12} \sum_{i=1}^N \sum_{j=0}^{i-1} \norm{\h^{\frac{1}{2}}\left(-\bm\mu_h +\langle q_h\n\rangle_t\right)}^2_{L^2(\Gamma_{ij})}\\
\ge & C_{12} \sum_{i=1}^N\sum_{j=0}^{i-1} \left(  \left(  \frac{C_{11}}{C_{12}} + 1 -\ell   \right) \norm{\h^{\frac{1}{2}} \langle q_h\rangle_t }^2_{L^2(\Gamma_{ij})}  + \left( 1-\frac{1}{\ell}\right) \norm{\h^{\frac{1}{2}} \bmu_h}^2_{L^2(\Gamma_{ij})}  \right).
\end{aligned}
\end{equation}
By plugging~\eqref{appendix:stress} back into~\eqref{appendix:hongkong}, we have
\begin{align*}
\overline{\mathcal A}_h&\left(\left( \vv_h + k \w^q_h,-q_h,-\bm\mu_h+\eta P_h \h^{-1} [\vv_h] \right) ;\left( \vv_h,q_h,\bmu_h\right)\right) \ge  \left( \frac{1}{2}-kC_4 -\eta C_8\right) \sum_{i=0}^N \norm{D\vv_i}^2_{L^2(\Omega_i)}\\
+& C_{12} \left( \frac{C_{11}}{C_{12}}+1 -\ell \right) \sum_{i=1}^N \sum_{j=0}^{i-1} \norm{\h^{\frac{1}{2}} \langle q_h  \rangle_t}^2_{L^2(\Gamma_{ij})} + \left( C_{12}\left(1-\frac{1}{\ell}\right) -k C_6\right) \sum_{i=1}^N\sum_{j=0}^{i-1} \norm{\h^{\frac{1}{2}} \bmu_h}^2_{L^2(\Gamma_{ij})} \\
+& \frac{kC}{4}\norm{q_h}^2_{0,h} + \frac{\eta}{2} \sum_{i=1}^N \sum_{j=0}^{i-1} \norm{\h^{-\frac{1}{2}} [\vv_h]}^2_{L^2(\Gamma_{ij})} .
\end{align*}
We require $\displaystyle 1<\ell < \frac{C_{11}}{C_{12}}+1$ and $k,\eta$ to be small enough so that $\displaystyle \frac{1}{2}-kC_4 -\eta C_8\ge \frac{1}{4}$, $\displaystyle C_{12} \left( \frac{C_{11}}{C_{12}}+1 -\ell \right) \ge C_{13}$, $\displaystyle C_{12}\left(1-\frac{1}{\ell}\right) -k C_6\ge C_{14}$, for some $C_{13}, C_{14}>0$. Note that the choice of $\ell$ depends on $k$ and $\eta$. On the other hand, there exist $C_{15},C_{16}>0$ such that $\displaystyle \frac{kC}{4}\ge C_{15}$ and $\displaystyle \frac{\eta}{2} \ge C_{16}$. Hence,
\begin{align*}
\overline{\mathcal A}_h&\left(\left( \vv_h + k \w^q_h,-q_h,-\bm\mu_h+\eta P_h \h^{-1} [\vv_h] \right) ;\left( \vv_h,q_h,\bmu_h\right)\right) \ge  \frac{1}{4} \sum_{i=0}^N \norm{D\vv_i}^2_{L^2(\Omega_i)}\\
+& C_{13} \sum_{i=1}^N \sum_{j=0}^{i-1} \norm{\h^{\frac{1}{2}} \langle q_h  \rangle_t}^2_{L^2(\Gamma_{ij})} + C_{14} \sum_{i=1}^N\sum_{j=0}^{i-1} \norm{\h^{\frac{1}{2}} \bmu_h}^2_{L^2(\Gamma_{ij})}\\
+& C_{15}\norm{q_h}^2_{0,h} +C_{16} \sum_{i=1}^N \sum_{j=0}^{i-1} \norm{\h^{-\frac{1}{2}} [\vv_h]}^2_{L^2(\Gamma_{ij})} .
\end{align*}
Finally, the stability property of $\w_h^q$, namely $\norm{\w_h^q}_{1,h}\le C \norm{q_h}_{0,h}$, entails
\begin{align*}
\vertiii{\left(\vv_h+k\w_h^q,-q_h,-\bm\mu_h+\eta P_h \h^{-1}[\vv_h]\right)}\le C  \vertiii{\left(\vv_h,q_h,\bm\mu_h\right)}.
\end{align*}
\end{proof}
%------------------------------------------------------------------------------------------------------------------------------
%------------------------------------------------------------------------------------------------------------------------------	
\IfStandalone
{
\bibliographystyle{../elsarticle-num}
\bibliography{../bibliographyx}
}{}

\end{document}
